# Supplementary material for: Remarkable Stability of Charge Density Wave Order in La$_{1.875}$Ba$_{0.125}$CuO$_4$
Source: arXiv:1606.04168 ancillary file (2018-03-04)
Supplement: Supplementary file 1 [file supplementary.pdf]

# Supplemental Material for: Remarkable Stability of Charge Density Wave Order in $\text{La}_{1.875}\text{Ba}_{0.125}\text{CuO}_4$

X. M. Chen,<sup>1,\*</sup> V. Thampy,<sup>1,†</sup> C. Mazzoli,<sup>2</sup> A. M. Barbour,<sup>2</sup> H. Miao,<sup>1</sup> G. D. Gu,<sup>1</sup> Y. Cao,<sup>1</sup> J. M. Tranquada,<sup>1</sup> M. P. M. Dean,<sup>1,‡</sup> and S. B. Wilkins<sup>2,§</sup>

<sup>1</sup>*Department of Condensed Matter Physics and Materials Science,  
Brookhaven National Laboratory, Upton, New York 11973, USA*

<sup>2</sup>*National Synchrotron Light Source II, Brookhaven National Laboratory, Upton, New York 11973, USA*

(Dated: September 14, 2016)

## 1. CALCULATION OF SPECKLE INTENSITY VARIATION

Here we reproduce the equations derived by Mark Sutton in Ref. [1] for calculating the expected speckle intensity variation, which depends on the beam properties and the scattering geometry. The beam is defined in terms of horizontal and vertical transverse x-ray coherence lengths  $\xi_h$  and  $\xi_v$ , as well as the beamline energy resolution  $\Delta\lambda/\lambda$ , which determines the longitudinal coherence length. Figure 1 defines the scattering angles. This assumes an idealized beamline and neglects possible contributions from the finite spatial resolution of the detector. Using this model, the speckle intensity variation  $V = \sqrt{\beta}$ , where  $\beta$  is the speckle contrast factor, which can be separated into two integral equations as

$$\beta = \beta_z \beta_r \quad (1)$$

where

$$\beta_z = \frac{2}{M^2} \int_0^M (M - z) e^{-z^2/\xi_v^2} dz \quad (2)$$

and

$$\beta_r = \frac{2}{W^2 L^2} \int_0^L (L - x) dx \int_0^W (W - y) e^{-x^2/\xi_h^2} \left[ e^{-|Ax+By|} + e^{-|Ax-By|} \right] dy. \quad (3)$$

This depends on parameters

$$A = \frac{4k_0 \Delta\lambda}{\lambda} [\cos(\theta) \sin(\theta) - \sin^2(\theta) \cot(\theta_i)] \quad (4)$$

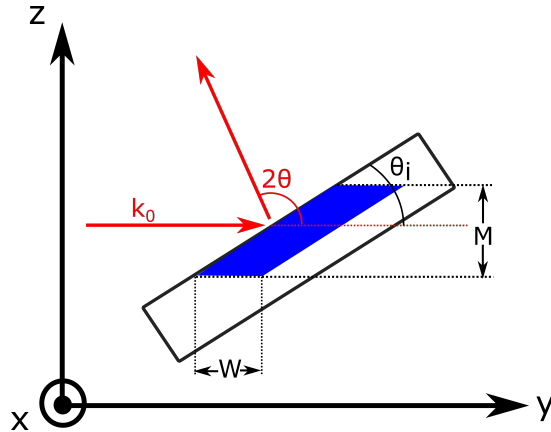

FIG. 1. X-rays with wavevector  $k_0$  are incident on the sample at angle  $\theta_i$  and are scattered through angle  $2\theta$ . The projections of the illuminated sample volume (shown in blue) along the  $y$  and  $z$  axes are  $W$  and  $M$ , respectively.

TABLE I. The measured values of the speckle intensity variation  $V = (I_s^{\max} - I_s^{\min}) / (I_s^{\max} + I_s^{\min})$  at 15 K compared to the calculated equivalent quantity  $\sqrt{\beta}$  for the different resonances and CDW peak satellites. Errorbars are determined by taking approximately 15 independent cuts through the CDW peak and calculating the standard error from the variation in the values.

|                                      | Cu $L$ -edge -H | Cu $L$ -edge +H | O $K$ -edge -H  | O $K$ -edge +H  |
|--------------------------------------|-----------------|-----------------|-----------------|-----------------|
| Measured speckle intensity variation | $0.15 \pm 0.05$ | $0.23 \pm 0.07$ | $0.18 \pm 0.05$ | $0.27 \pm 0.09$ |
| Calculated $\sqrt{\beta}$            | 0.15            | 0.21            | 0.13            | 0.21            |

and

$$B = \frac{-4k_0\Delta\lambda}{\lambda} \sin^2(\theta) , \quad (5)$$

which depend on the incident x-ray angle  $\theta_i$  and the angle of the scattered x-rays  $2\theta$ .

In the measurements reported here, the beamline was configured with  $\xi_h = \xi_v = 10 \text{ } \mu\text{m}$  and  $\Delta\lambda/\lambda \approx 1/1900$ .  $M = 10 \text{ } \mu\text{m}$  was determined by the pinhole, whereas  $W$  is determined by the x-ray penetration depth along the beam. At the Cu  $L_3$  edge  $W = 0.15 \text{ } \mu\text{m}$  and  $2\theta = 119^\circ$  with  $\theta_i = 88^\circ$  or  $\theta_i = 31^\circ$  for the positive and negative  $H$  satellites. Corresponding values for the O  $K$ -edge are  $W = 0.24 \text{ } \mu\text{m}$  and  $2\theta = 141^\circ$  with  $\theta_i = 121^\circ$  or  $\theta_i = 20^\circ$ .

Table I compares the measured and calculated speckle intensity variation for the four CDW measurement configurations. The calculations capture the reduced speckle intensity variation at higher incident energies and smaller incident angles. All measured values are within the errorbar and we therefore conclude that the observed speckle visibility is consistent with what is expected based on the known beamline configuration and geometrical considerations.

## 2. MODEL FOR $\beta$ SCALING WITH CONSTANT BACKGROUND

Here we construct a simple model for the variation in the speckle contrast,  $\beta$ , in the presence of a constant incoherent background intensity,  $B$ . To model this we assume an average x-ray intensity,  $I$ , is modulated depending on the size of  $V$ , the speckle intensity variation, such that the minimum and maximum intensity is  $I(1 - V)$  and  $I(1 + V)$ . The intrinsic speckle contrast factor,  $\beta_i$ , that is obtained when  $B = 0$ , can be determined from  $g_2(\tau)$ , as defined in the main text. Labeling each intensity point by index  $j$ , we can write

$$\beta_i = g_2(\tau \rightarrow 0) - 1 = \frac{\langle I_j^2 \rangle}{\langle I_j \rangle^2} - 1. \quad (6)$$

Assuming equal occurrences of  $(1 + V)I$  and  $(1 - V)I$ , we obtain

$$\beta_i = V^2 \quad (7)$$

In the presence of non-zero incoherent background intensity we add  $B$ , to  $I$  in Eq. 6 above, and define  $r = I/(I+B)$ , to obtain

$$\beta = r^2 V^2 = r^2 \beta_i, \quad (8)$$

where  $\beta$  is the speckle contrast factor after accounting for the constant background.

## 3. EXPERIMENTAL STABILITY TIMESCALE

In the main article, we attribute the small drop in  $g_2(\tau)$  at 15 and 30K (main text Fig. 4) to finite experimental stability. This was inferred by tracking the time evolution of a speckle pattern from a sample with known static disorder. The specular reflection from a piece of chemically roughened pyrex glass yielded such a speckle pattern which is expected to be totally static. Therefore, any time evolution of the speckle pattern, as indicated by a decay in  $g_2(\tau)$ , directly reflects finite experimental stability.

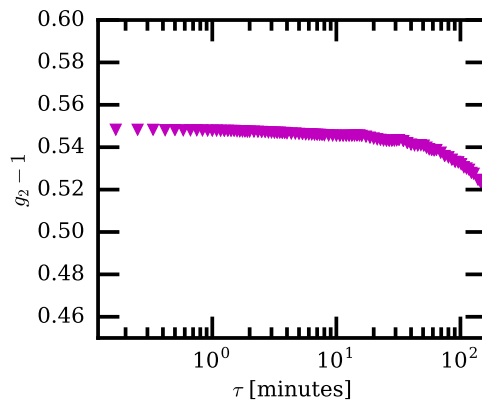

FIG. 2. One-time correlation function of a specular reflection from a corrugated glass piece as a function of time. The resulting speckle pattern is expected to be static. So the decay in  $g_2$  reflects the finite experimental stability.

Figure 2 shows the measured  $g_2(\tau)$  for the glass sample over a similar timescale as plotted in Fig. 4. We find that the overall stability is sufficient to study sample dynamics on the timescale of hours and we anticipate further improvements at the CSX beamline to extend this timescale in the future. The decay in  $g_2$  for this expected static speckle pattern is found to occur at a comparable timescale as that observed for the measured CDW peak. This allows us to assign the downturn in  $g_2$  seen in Fig. 4 to finite experimental stability.

---

\* xmchen@bnl.gov; Contributed equally to this work

† vthampy@bnl.gov; Contributed equally to this work

‡ mdean@bnl.gov

§ swilkins@bnl.gov

- [1] M. Sutton, “Coherent x-ray diffraction,” in *Third-Generation Hard X-ray Synchrotron Radiation Sources: Source Properties, Optics, and Experimental Techniques*, edited by D. M. Mills (John Wiley and Sons, New York, 2002).
